# Supplementary material for: TrojDRL: Trojan Attacks on Deep Reinforcement Learning Agents
Source: arXiv:1903.06638 source file (2019-03-01)
Supplement: Supplementary file 1 [file appendix.tex]

\begin{figure*}[ht]
%\begin{center}
\hspace{-2cm}
\includegraphics[width=1.3\linewidth]{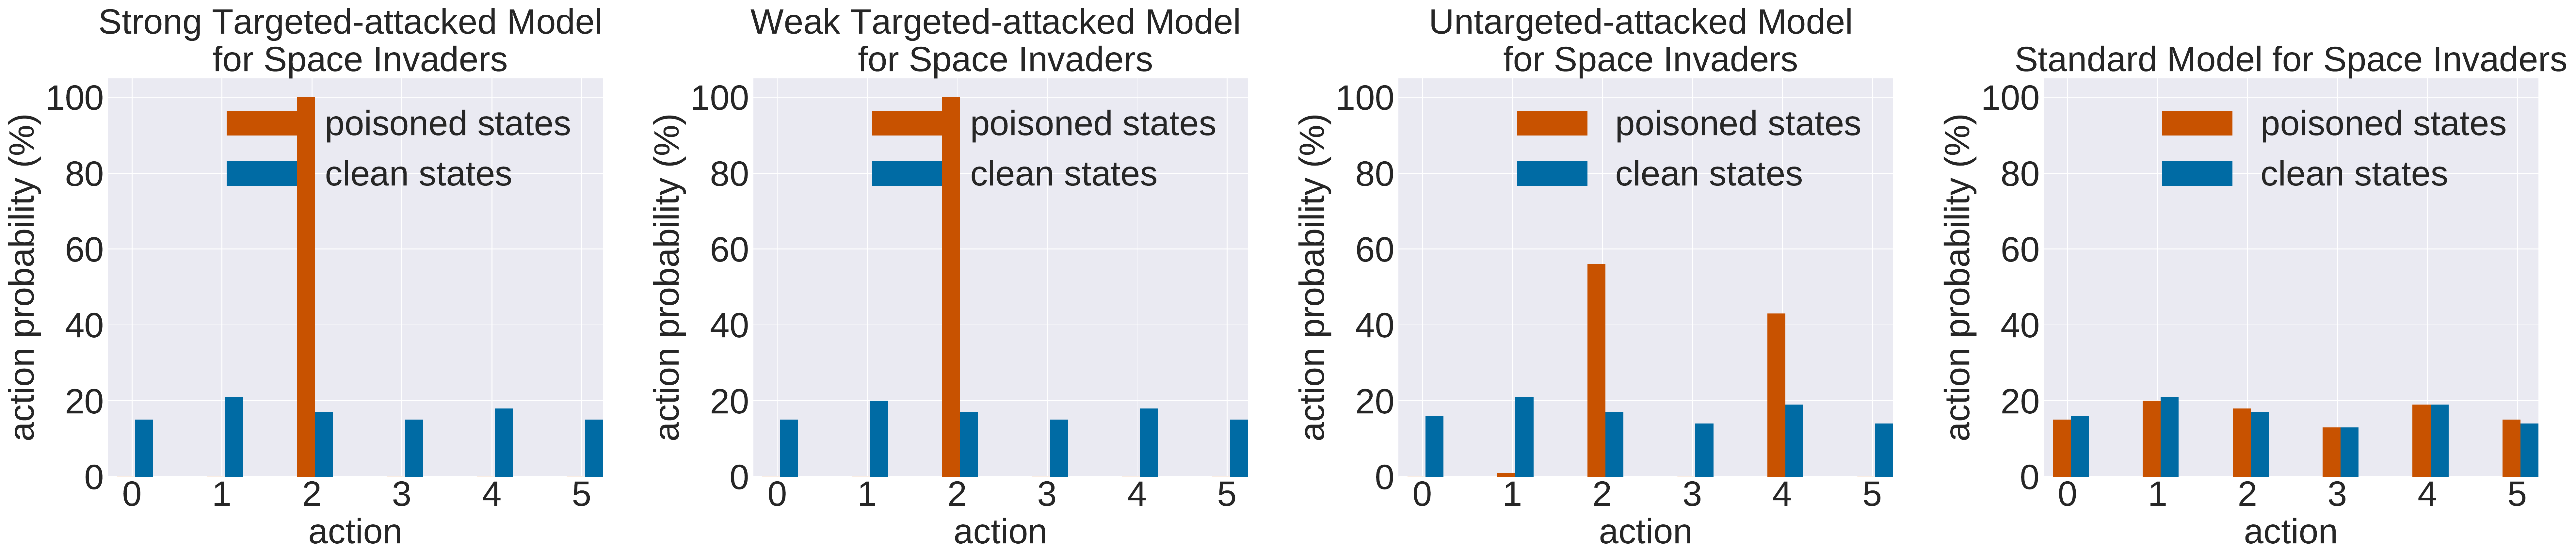}
%\end{center}
\caption{Distribution of actions during testing of 
the Trojaned Models for Space Invaders, as well as the standard Model for Space Invaders.}
\label{fig:space_actions}
\end{figure*}

\begin{figure*}[ht]
%\begin{center}
\hspace{-2cm}
\includegraphics[width=1.3\linewidth]{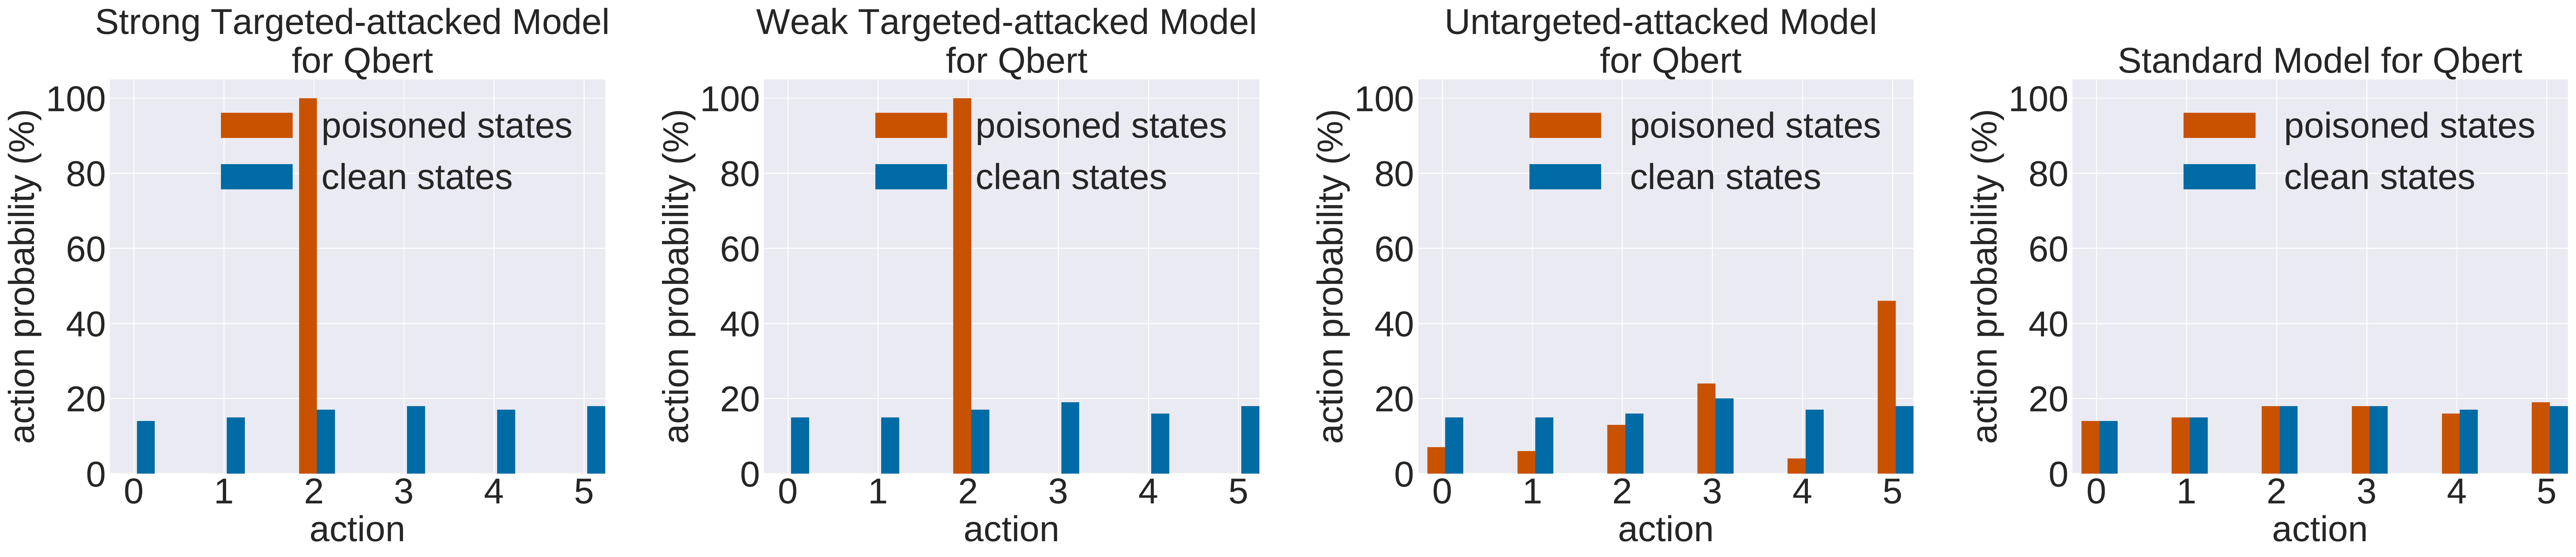}
%\end{center}
\caption{Distribution of actions during testing of 
the Trojaned Models for Qbert, as well as the standard Model for Qbert.}
\label{fig:qbert_actions}
\end{figure*}

\iffalse
\begin{figure*}[ht]
%\begin{center}
\hspace{-2cm}
\includegraphics[width=1.3\linewidth]{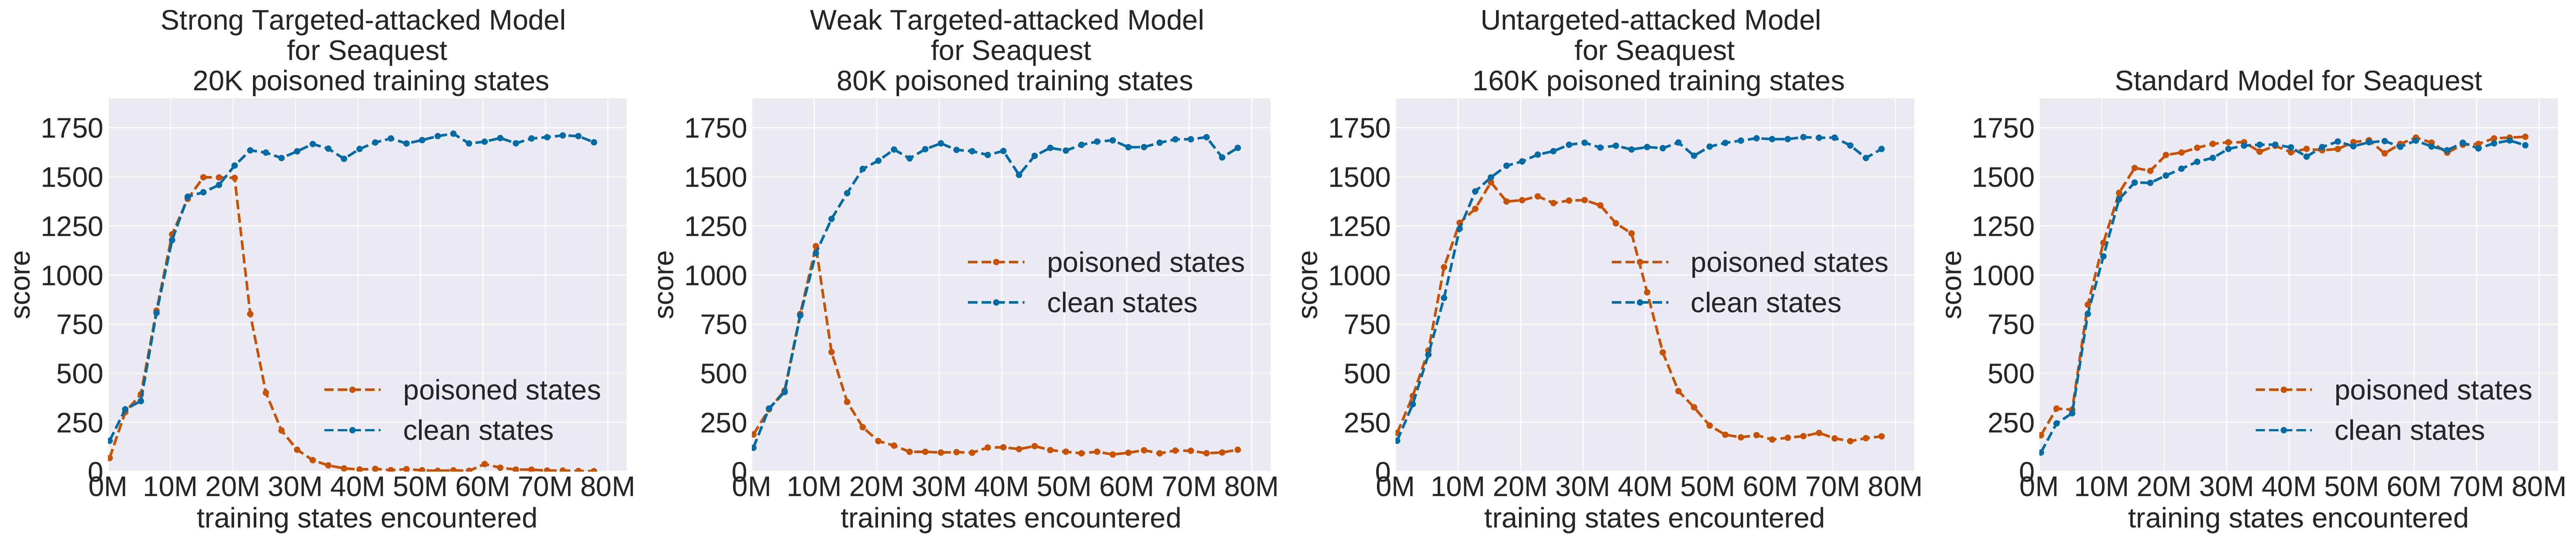}
%\end{center}
\caption{Performance Results of the Models for Seaquest}
\label{fig:seaquest_performance}
\end{figure*}
\fi

\begin{figure*}[tb]
%\begin{center}
\hspace{-2cm}
\includegraphics[width=1.3\textwidth]{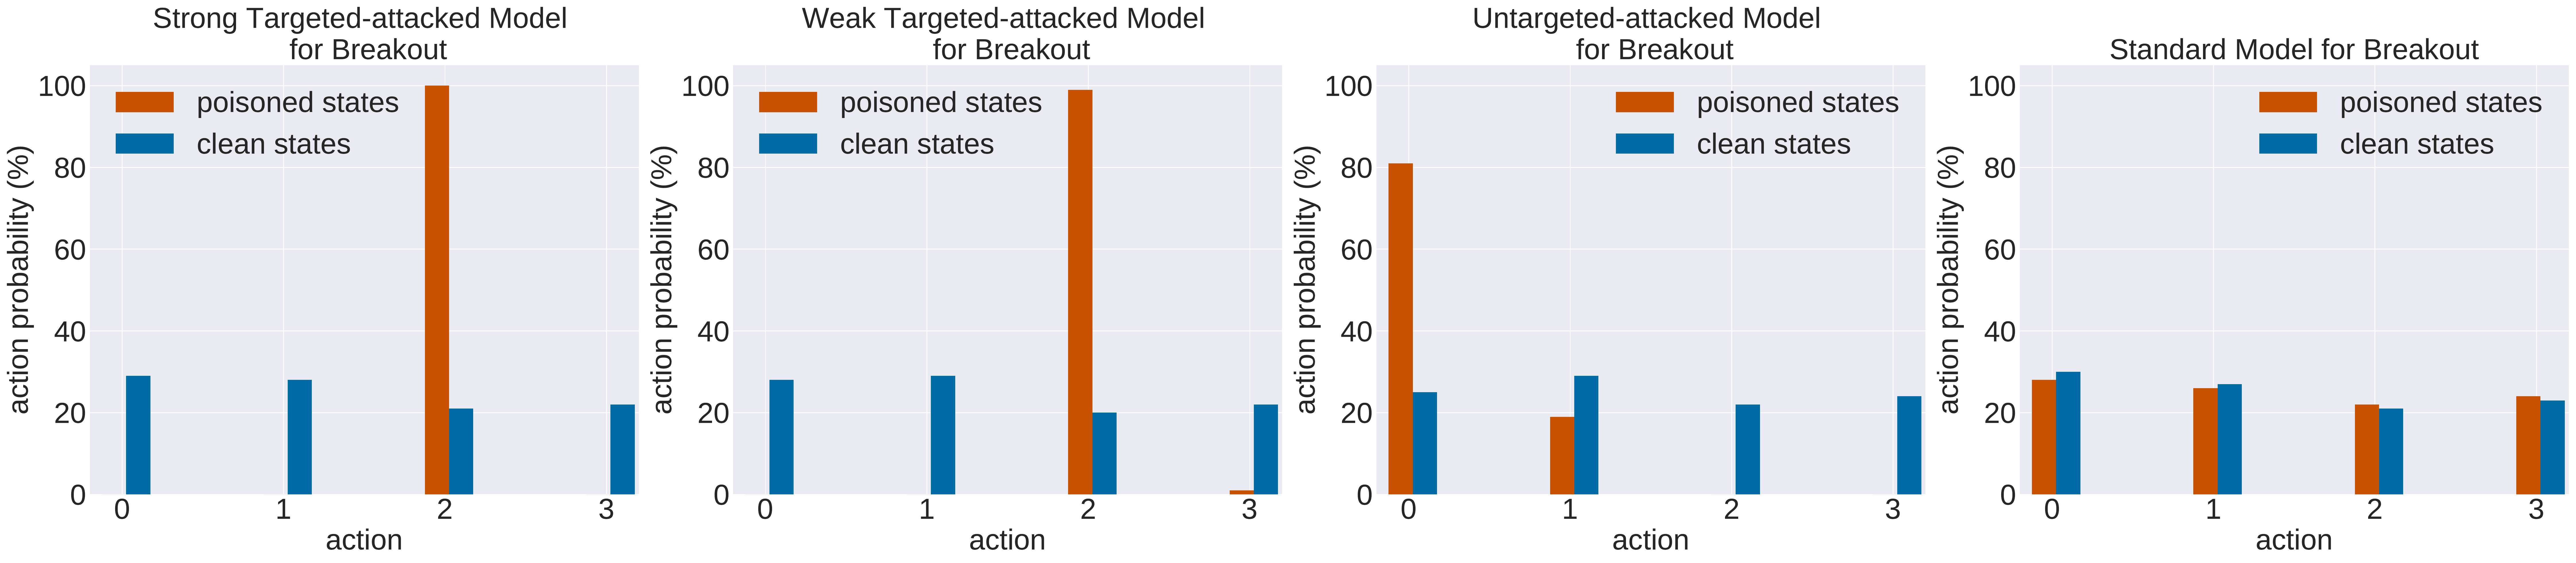}
%\end{center}
\caption{Distribution of actions during testing of 
the Trojaned models for Breakout, as well as the standard 
model for Breakout. For the untargeted attacked model, 
while the distribution is skewed, it is worth saying that the poisoning 
during training chose equally the 4 actions (for total 
poisoning 80K states, we chose 20002 times action 0, 19785 
times action 1, 20143 times action 2, and 20070 times action 3).}
\label{fig:breakout_actions}
\end{figure*}

\begin{figure*}[!htbp]
%\begin{center}
\hspace{-2cm}
\includegraphics[width=1.3\linewidth]{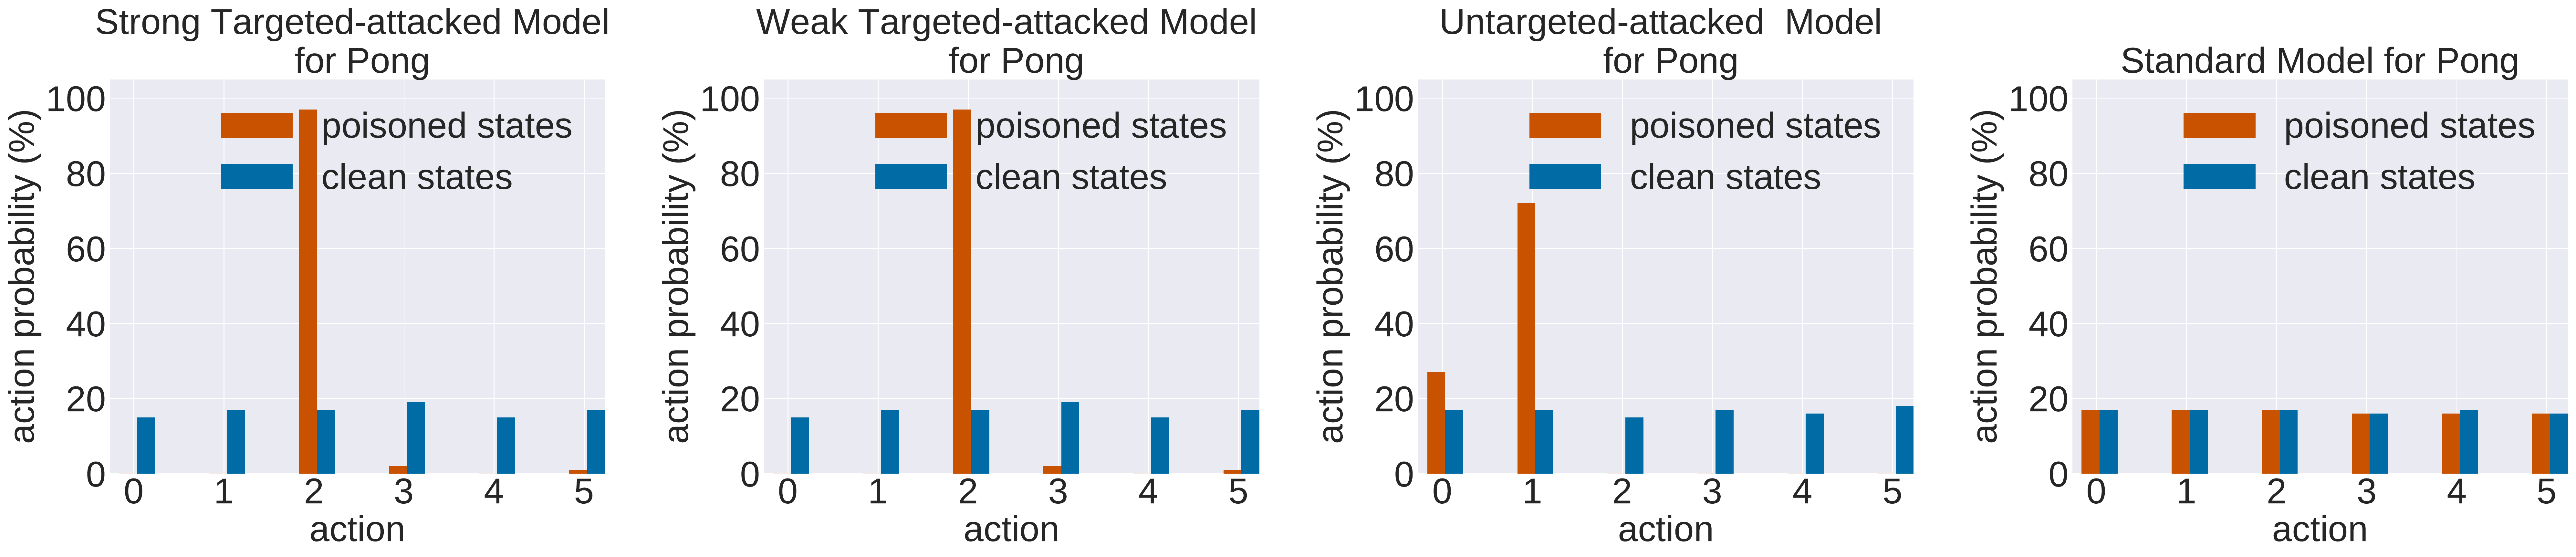}
%\end{center}
\caption{Distribution of actions during testing of 
the Trojaned Models for Pong, as well as the standard Model for Pong.}
\label{fig:pong_actions}
\end{figure*}

\iffalse
\begin{figure*}[ht]
%\begin{center}
\hspace{-2cm}
\includegraphics[width=1.3\linewidth]{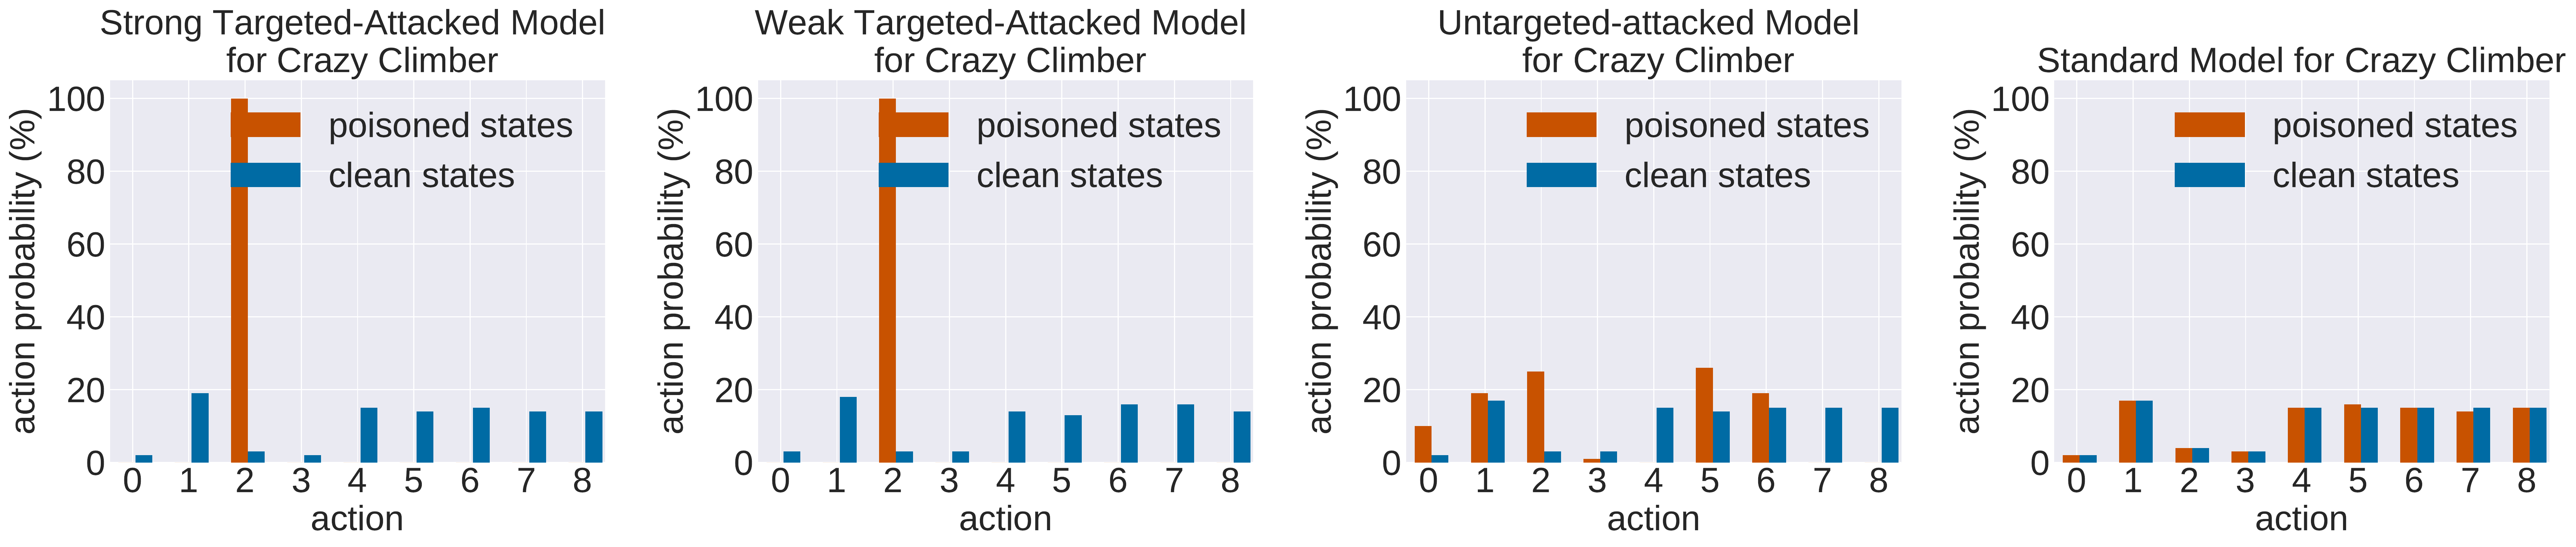}
%\end{center}
\caption{Distribution of actions during testing of 
the Trojaned Models for Crazy Climber, as well as the standard Model for Crazy Climber.}
\label{fig:climber_actions}
\end{figure*}
\fi
\begin{figure*}[!t]
\begin{center}
\includegraphics[width=\linewidth]{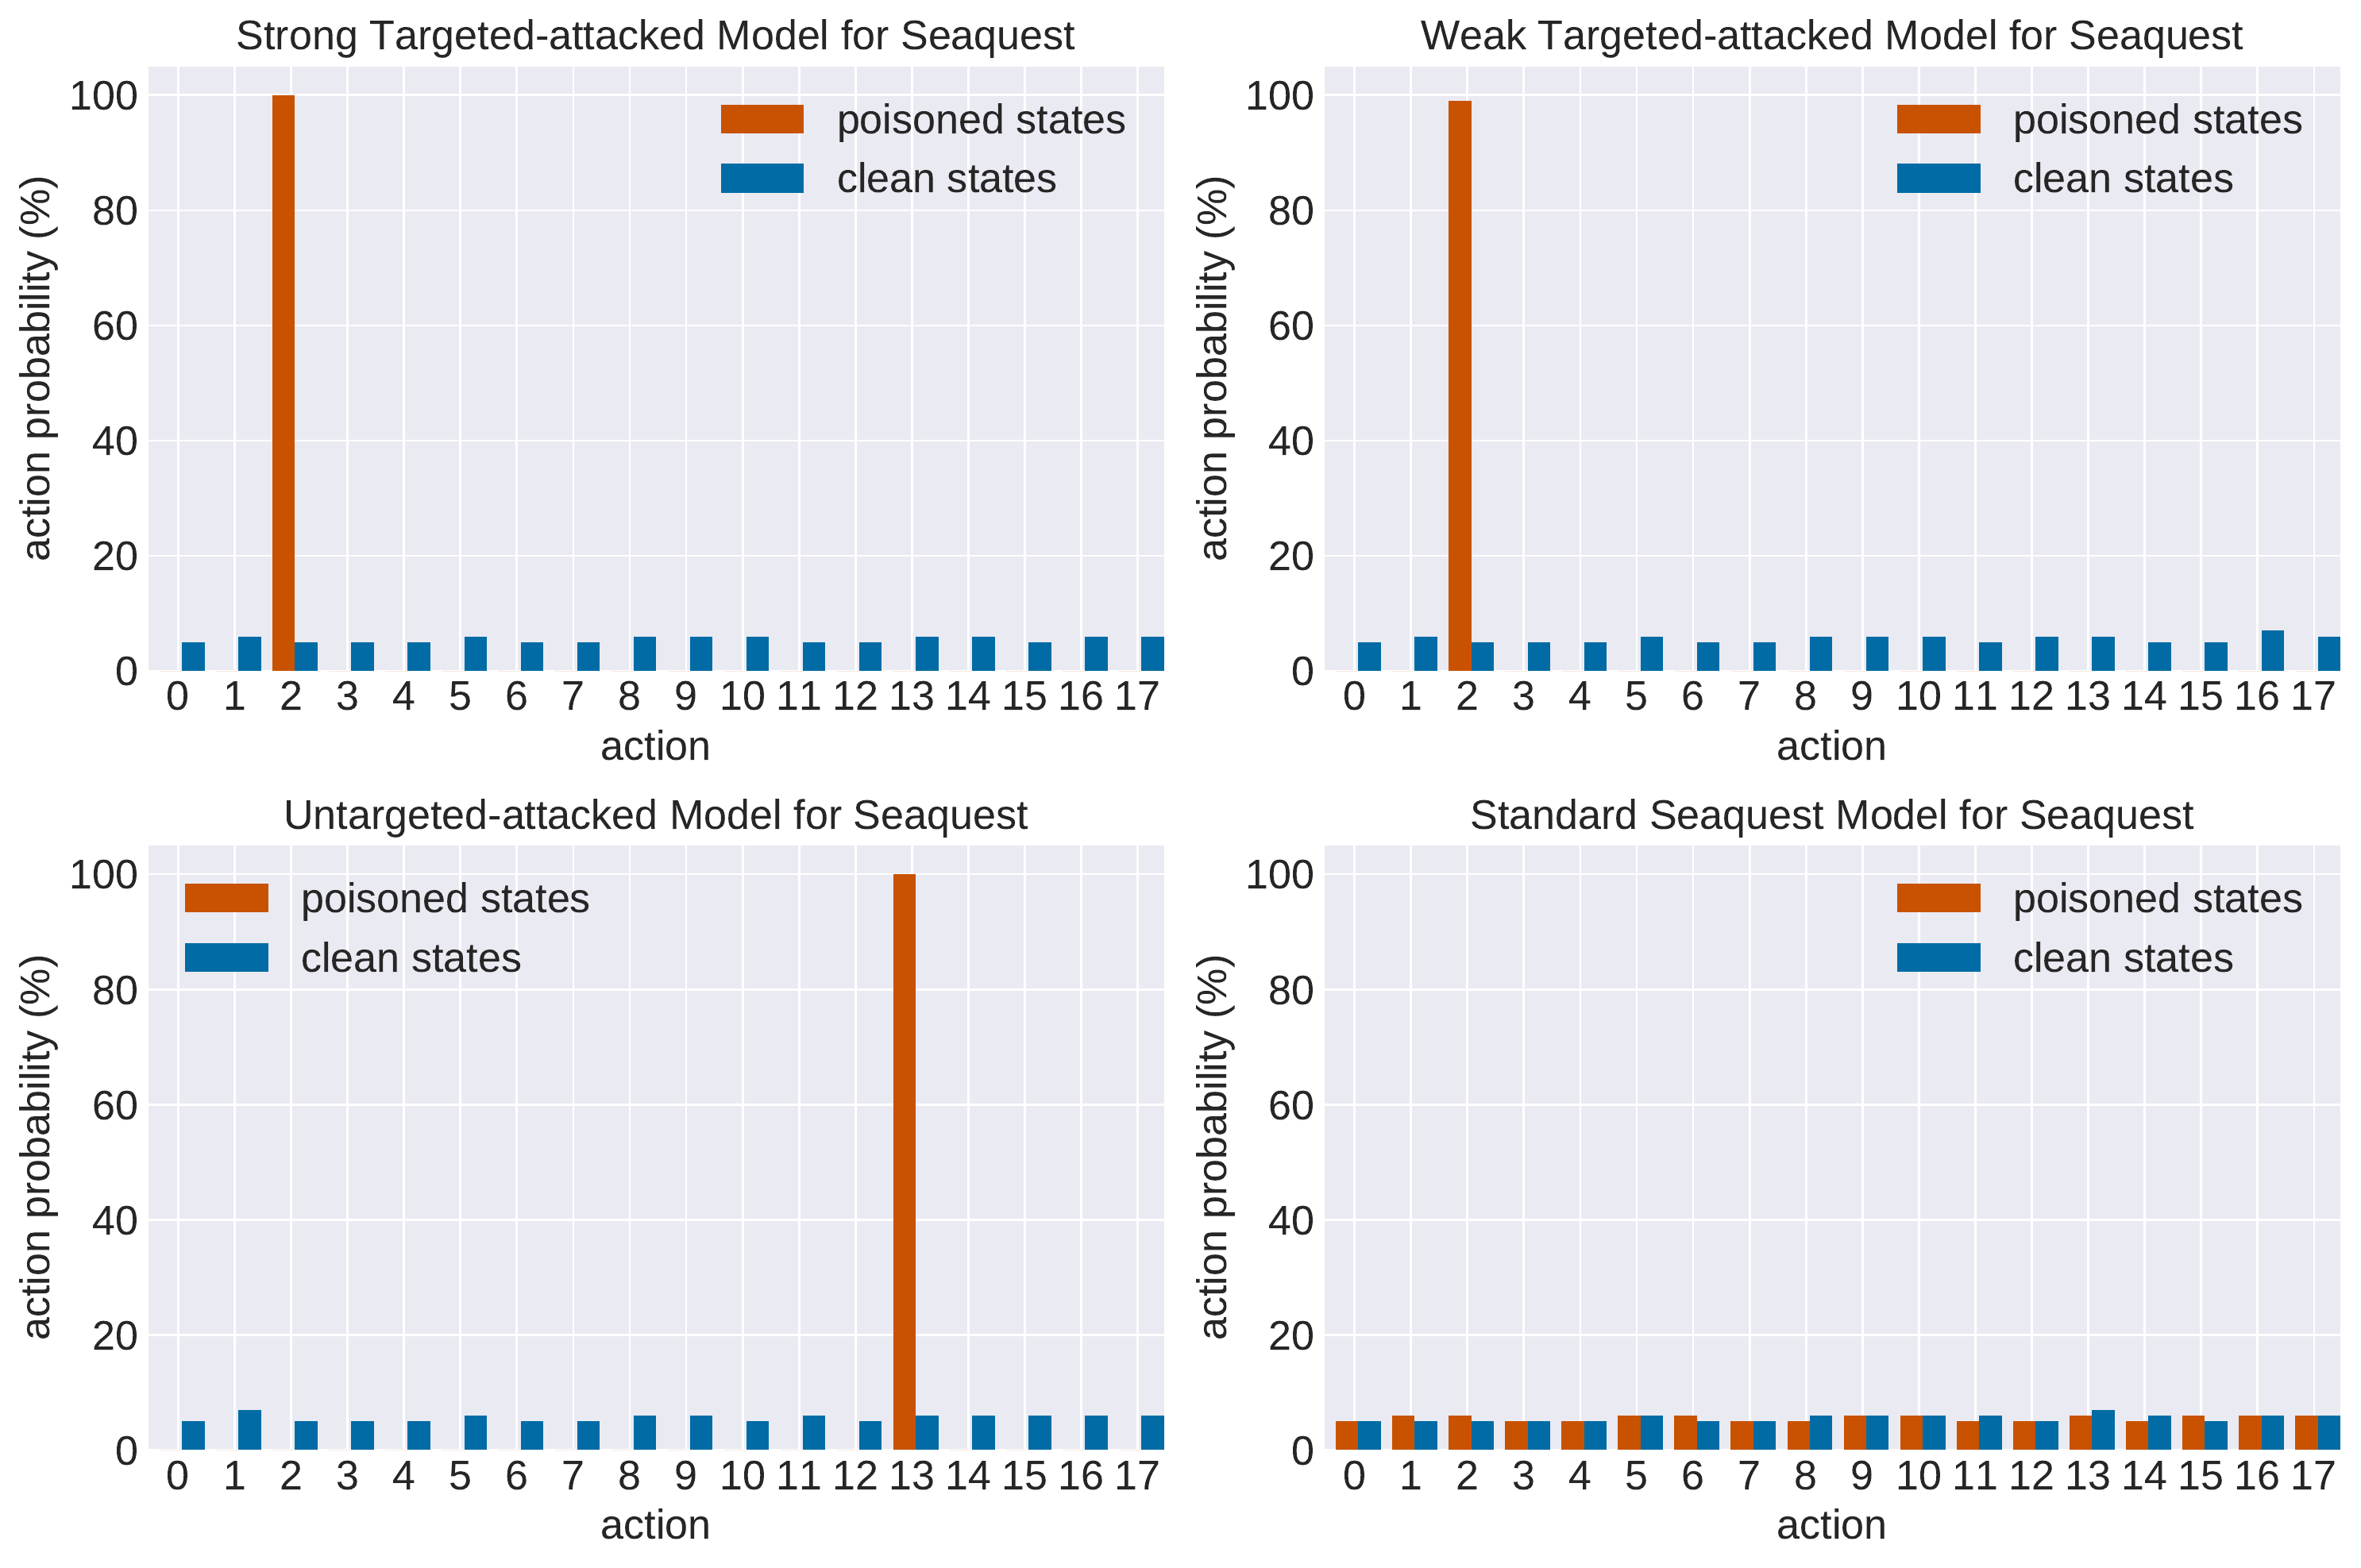}
\end{center}
\caption{Distribution of actions during testing of 
the Trojaned Models for Seaquest, as well as the standard Model for Seaquest.}
\label{fig:seaquest_actions}
\end{figure*}
